# Supplementary material for: RTLSquad: Multi-Agent Based Interpretable RTL Design
Source: arXiv:2501.05470 source file (2025-01-06)
Supplement: Supplementary file 1 [file appendix.tex]

\section{Detailed Experimental Setup}
\label{sec:appendix_setup}
